# Supplementary material for: Dynamics and transport of Bose-Einstein condensates in bent potentials
Source: arXiv:2508.17383 ancillary file (2025-08-24)
Supplement: Supplementary file 1 [file Supplementary_material.pdf]

# Dynamics and transport of Bose-Einstein condensates in bent potentials (Supplementary material)

Rhombik Roy[1,2,*] and Ofir E. Alon[1,2]

[1]Department of Physics, University of Haifa, Haifa 3498838, Israel

[2]Haifa Research Center for Theoretical Physics and Astrophysics, University of Haifa, Haifa 3498838, Israel

In this supplementary material, we provide additional analysis to support and enrich the findings presented in the main text. We begin by examining the depletion dynamics, which reveal the emergence of many-body effects during the transport. By comparing different parameters of the bent potential, we identify regimes of self-trapping, partial tunneling, and full transport, thereby illustrating how the buildup of correlations manifest in those configurations using the depletion dynamics. Next, we study the survival probability as a diagnostic of the tunneling dynamics and controlled transport. Studying the survival probability within this framework offers further insight into the transport mechanisms enabled by geometric control. The connection between the survival probability and the expectation value of the position operator are briefly discussed. Finally, we discuss the convergence analysis of the numerical simulations, focusing on two key aspects: the number of time-adaptive orbitals employed in the many-body calculations, and the resolution of the spatial grid. Both factors are examined in detail to ensure the accuracy of the results.

## I. DEPLETION DYNAMICS

To probe the role of the geometry in controlling the many-body effects, we analyze in detail the depletion dynamics associated with transport through the bent potential for three different control scenarios: variation of the half-width of the bent $B$ [Fig. S1(a)], the sharpness of the bent $D$ [Fig. S1(b)], and the transverse confinement $a$ [Fig. S1(c)]. The corresponding $\langle x \rangle$ and $\langle y \rangle$ are discussed in the main text.

The reduced one-body density matrix (RDM) can be constructed from the wave-function $|\Psi(t)\rangle$ as

$$\rho^{(1)}(\mathbf{r}, \mathbf{r}') = \langle \Psi | \hat{\Psi}(\mathbf{r}') \hat{\Psi}(\mathbf{r}) | \Psi \rangle = \sum_j n_j \alpha_j(\mathbf{r}) \alpha_j^*(\mathbf{r}'). \tag{1.1}$$

* rroy@campus.haifa.ac.il

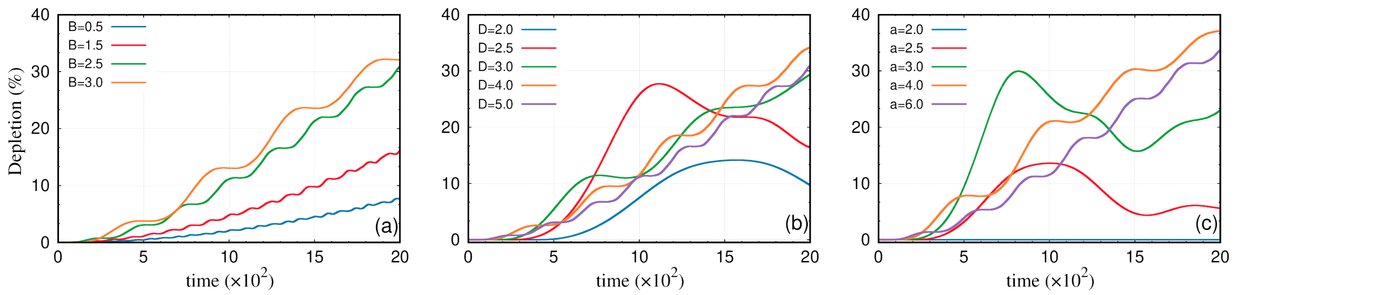


FIG. S1. Time evolution of the depletion for different geometric parameters of the bent potential. Depletion dynamics (a) for different half-width of the bent $B$, at fixed $D = 5.0$ and $a = 7.0$; (b) for different sharpness of the bent $D$, at fixed $B = 2.5$ and $a = 7.0$; and (c) for different transverse confinement $a$, at fixed $B = 2.5$ and $D = 5.0$. In all cases, the system evolves from a highly condensed initial state, with depletion growing over time. All quantities are dimensionless. See text for more details.

Where $n_j$ is the $j-$th eigenvalues and $\alpha_j(\mathbf{r})$ are the natural orbitals. The diagonal part of the one-body RDM, i.e., $\rho^{(1)}(\mathbf{r}, \mathbf{r})$ gives the one-body density which is denoted as $\rho(x, y)$. For a condensed system, the RDM has only one macroscopic eiganvalue and the system is called fragmented when more than one macroscopic eiganvalues exist [1–4]. Thus, $\frac{n_1}{N} \simeq 1$ corresponds to condensed system and $\frac{n_1}{N} < 1$ applies to the fragmented system. The amount of fragmentation can be measured in terms of the depletion which is denoted by Depletion% $= (1 - n_1) \times 100$.

Figure S1(a) shows the depletion dynamics for different half-widths of the bent, with the other parameters held fixed at $D = 5.0$ and $a = 7.0$. When the bent width is small ($B = 0.5$), the system exhibits oscillations with a shorter time period (see Fig. 4 of the main text), and the depletion grows slowly with time. This behavior reflects a coherent, mean-field-like evolution where the amplitude of many-body expectation values shows minimal decay over time, and the variances nearly overlap with mean-field results (see the main text; Figs. 4, 5). However, at longer times, noticeable deviations emerge between the mean-field and many-body position variances, driven by the substantial buildup of depletion. As $B$ increases, the oscillations becomes more regular with longer time periods, leading to rapid growth in depletion over time. This also results in the prominent decay of the oscillations' amplitude of the many-body expectation values, and significant deviations between mean-field and many-body position variances are observed even from the early-time dynamics (shown in the main text).

Figure S1(b) illustrates how the sharpness of the bent ($D$) affects the depletion dynamics with the other parameters held fixed at $B = 2.5$ and $a = 7.0$. When the bent is sharp ($D = 2$), the initially highly condensed system exhibit partial transport, as demonstrated in the main text

(see Fig. 6). This results in slow increase in the depletion over time and a correspondingly small maximum depletion value. As the sharpness of the bent decreases with increasing $D$, the depletion grows at a faster rate. For $D = 2.5$, complete oscillations are observed, but the extremely long time period produces depletion behavior that differs substantially from other cases. At higher $D$ values, the depletion exhibits consistent increase over time.

Fig. S1(c) shows how the transverse confinement of the bent affects the depletion dynamics, with the other parameters held fixed at $D = 5.0$ and $B = 2.5$. When the transverse confinement is tight ($a = 2$), the system exhibits almost no transport (see Fig. 6 of the main text) and the initially highly condensed state remains nearly fully condensed. For $a = 2.5$, partial transport is observed which results in slow increase of depletion over time and a small maximum value of the depletion. As the transverse confinement becomes smoother with increasing $a$, the depletion grows at a faster rate. For $a = 3$, complete oscillations occur; however, the extremely long period leads to a depletion dynamics that differs from the other cases. At larger $a$ values, the depletion increases steadily over time.

By analogy with a conventional double well, the bent geometry defines an effective tunneling barrier. Adjusting the geometric parameters tunes the barrier height, which in turn controls the tunneling timescale and the onset of coherence loss. Still, the analogy is only approximate, because higher modes influence the transport and the system retains some angular momentum.

## II. SURVIVAL PROBABILITY

In this section, we analyze the transport in the bent potential through the measure of the survival probability. This concept arises naturally, as the back-and-forth motion between the two sides of the bent potential resembles the tunneling behavior typically observed in a double-well system. Since the effective double well generated because of the bent is not aligned along a single axis, oscillations occur along both the x- and y-directions. We therefore define survival probabilities for each spatial direction separately. The survival probability in the x-direction is defined as the fraction of particles remaining on the left side of the potential:

$$\mathcal{P}_x(t) = \frac{1}{N} \int_{y=-\infty}^{y=+\infty} \int_{x=-\infty}^{x=0} \rho(x, y; t) dx dy, \tag{2.1}$$

where $\rho(x, y; t)$ is the time-dependent density and $N$ is the total number of particles. Similarly, the survival probability in the y-direction is defined as the fraction of particles in the upper half

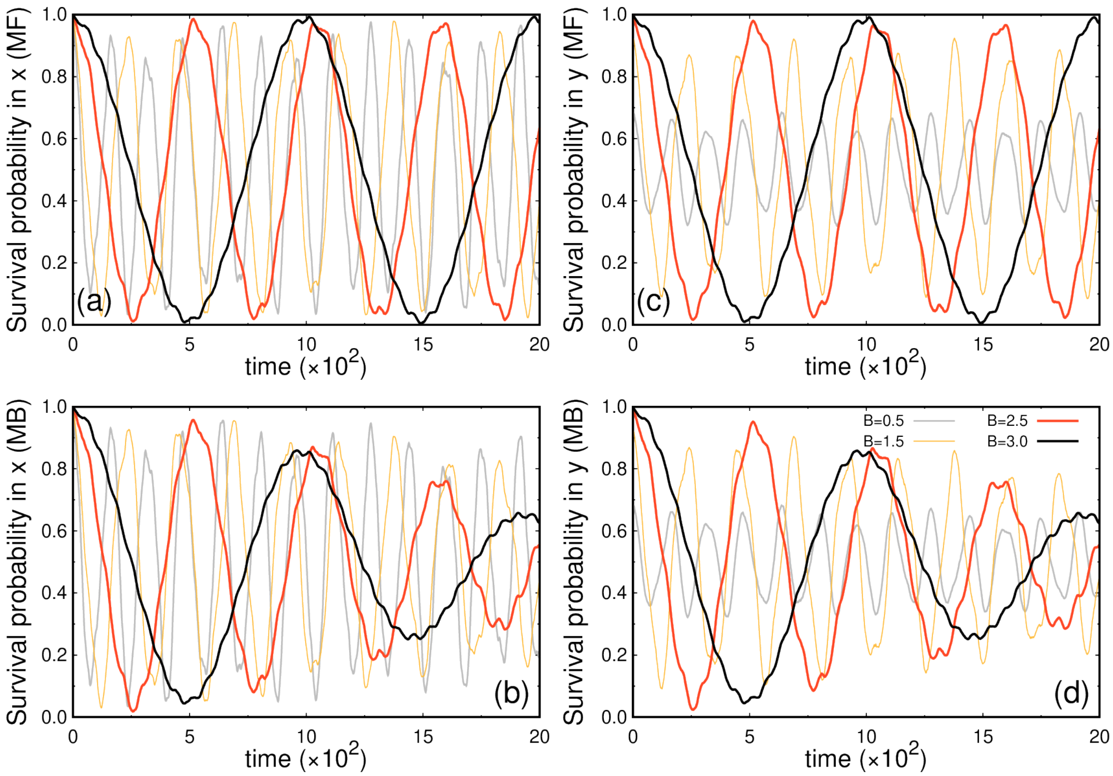


FIG. S2. Time evolution of the survival probabilities $\mathcal{P}_x(t)$ (left) and $\mathcal{P}_y(t)$ (right) for different half-widths of the bent $B$, comparing mean-field (MF, top) and many-body (MB, bottom) dynamics. Small $B$ yields fast oscillations, while larger $B$ leads to slower and more regular tunneling. The color codes are explained in the plot. The quantities shown are dimensionless.

of the potential:

$$\mathcal{P}_y(t) = \frac{1}{N} \int_{x=-\infty}^{x=+\infty} \int_{y=0}^{y=\infty} \rho(x, y; t) dx dy. \tag{2.2}$$

Figure S2 shows the time evolution of the survival probabilities $\mathcal{P}_x(t)$ and $\mathcal{P}_y(t)$ for different half-widths of the bent $B$, comparing mean-field (MF, panels a and c) and many-body (MB, panels b and d) results. For small widths ($B = 0.5$ and 1.5), the system exhibits oscillations with short time period, as quoted in the main text (Fig 4). As $B$ increases, the oscillations become smoother and the time period also increases. The many-body dynamics display a clear reduction in the amplitude of the oscillations compared to the mean-field case, reflecting the onset of fragmentation as discussed in the previous section. The survival probabilities along the x- and y-directions remain synchronized over time.

Figure S3 illustrates the time evolution of the survival probabilities $\mathcal{P}_x(t)$ and $\mathcal{P}_y(t)$ for different sharpnesses and transverse confinements of the bent. Panels (a,b) display the effect of varying the sharpness of the bent $D$, while panels (c,d) show the influence of the transverse confinement $a$.

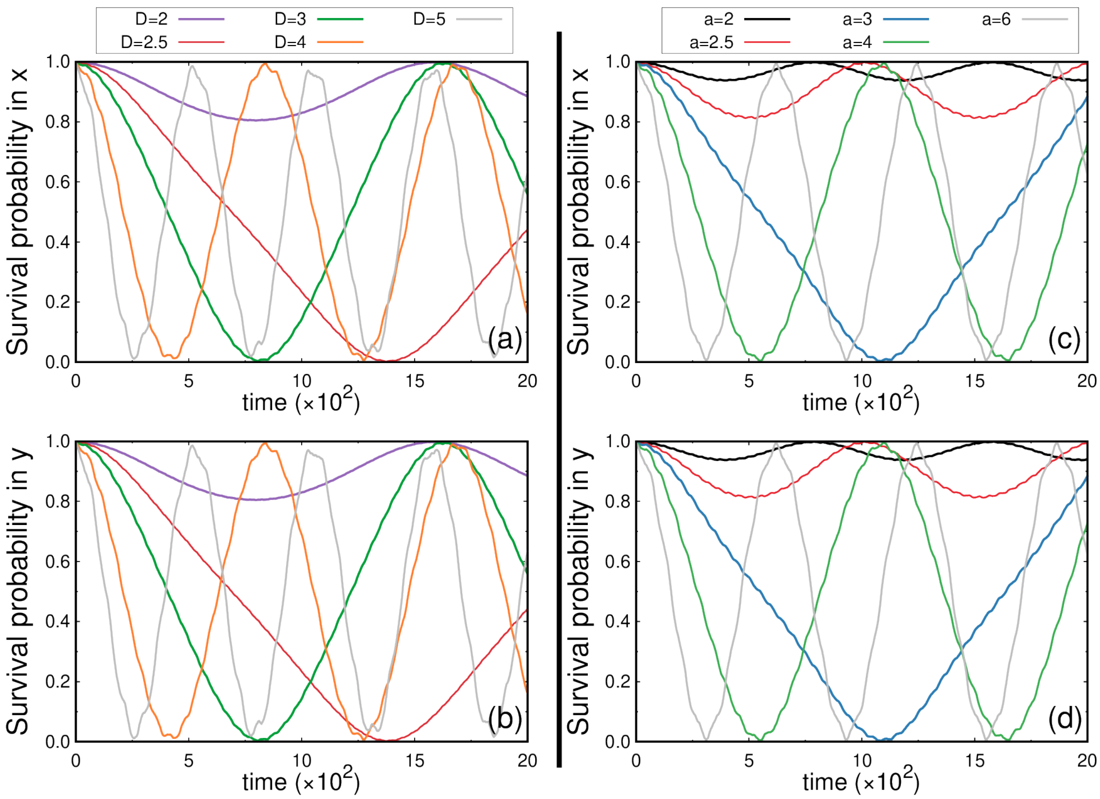


FIG. S3. Time evolution of the survival probabilities $\mathcal{P}_x(t)$ (top) and $\mathcal{P}_y(t)$ (bottom) in the bent potential, illustrating tunneling dynamics along the x- and y-directions. Panels (a,b) show the effect of varying the sharpness of the bent $D$ and panels (c,d) show the influence of the transverse confinement $a$. For sharp bent (small $D$) or narrow confinement (small $a$), the survival probability exhibits suppressed transport. Increasing $D$ or $a$ leading to complete oscillations whose periods decrease with further increase in $D$ or $a$. The color codes are explained in the plot. The quantities shown are dimensionless.

For small $D$ ($D = 2$), the survival probability remains relatively close to unity throughout the time evolution, indicating strong self-trapping and minimal transport. Increasing $D$ enhances the coupling between the sides of the bent, leading to complete oscillations. For $D = 2.5$ and $D = 3$, the oscillations occur with periods of approximately $T \approx 2700$ and 1600, respectively, while larger values $D = 4$ and $D = 5$ lead to faster oscillations ($T \approx 850$ and 525, respectively). Panels (c) and (d) illustrate the influence of the transverse confinement $a$ on the tunneling dynamics. Narrow confinement ($a = 2$ and 2.5) strongly suppresses the transport, mimicing the effects observed in the small $D$ regime. Increasing $a$ promotes the transport. For $a = 3$ and $a = 4$, the oscillations are complete with periods $T \approx 2180$ and 1090. The largest confinement width, $a = 6$, leads to the fastest oscillations ($T \approx 620$). Overall, these findings reveal a clear dynamical crossover: smoother bents and weaker transverse confinements allow for full coherent tunnelling. In contrast, sharper

bents and tighter confinements enhance localization which leads to self-trapping and suppressed tunnelling.

## III. CONVERGENCE OF THE OUT-OF-EQUILIBRIUM DYNAMICS AND ITS ANALYSIS

This section presents the convergence analysis of the results discussed in the main text. Achieving convergence in many-body dynamics is more challenging than in ground-state calculations, as the dynamics involve contributions from many excited states [5–7]. Therefore, we have demonstrated convergence specifically for the dynamics, which inherently ensures the convergence of the ground-state results as well (if one analyzes the results at $t = 0$). Also, in the bent potential, selecting an appropriate number of grid points is also crucial for accurately representing the bent. Therefore, we examine the convergence with respect to both the number of grid points and the number of time-adaptive orbitals in the many-body calculations.

We choose the half-width of the bend as $B = 2.5$, the sharpness as $D = 5.0$, and the transverse confinement as $a = 7.0$ to demonstrate the convergence of the many-body results. These intermediate values capture the essential physics of the system, where geometric effects become nontrivial. In this regime, the tunneling coupling between the two sides is relatively weak but still sufficient to allow full transport without suppressing tunneling. This regime also exhibits noticeable many-body features such as the buildup of depletion, making it ideal for assessing the convergence of the many-body results.

Figure S4 demonstrates the convergence of our many-body dynamics with respect to both the number of time-adaptive orbitals and the spatial grid resolution. In panel (a) we compare the occupation of the first four natural orbitals obtained using $M = 4$ and $M = 8$ time-adaptive orbitals. The results show an excellent agreement between the two simulations, with all occupation numbers from the $M = 4$ calculation lying on top of those from the $M = 8$ calculation. This confirms that $M = 4$ orbitals are sufficient to accurately capture the many-body dynamics.

Panel (b) presents the convergence analysis with respect to the grid resolution, comparing simulations using $128 \times 128$ and $256 \times 256$ grid points. The occupation in the natural orbitals obtained from both grid resolutions exhibit excellent agreement, confirming that the $128 \times 128$ grid points are sufficient to resolve the relevant spatial features of the curvature of the bent potential. This is especially crucial for our system, where spatial resolution must be fine enough to capture the geometry-induced features while maintaining computational efficiency.

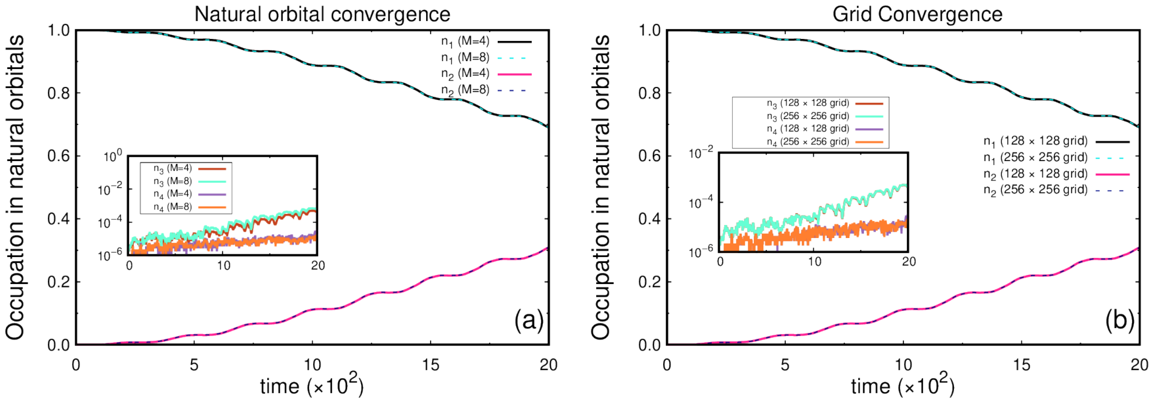


FIG. S4. (a) The convergence is analyzed with respect the number of natural orbitals. The occupation of the four natural orbitals are plotted for calculations with $M = 4$ and $M = 8$ time-adaptive orbital. All calculations with $M = 4$ falls on top of the $M = 8$ orbitals calculations. (b) The convergence is tested with respect to the number of grid points. The occupation of the four natural orbitals are plotted for calculations with $128 \times 128$ and $256 \times 256$ grid points in two spatial directions. The calculation with $128 \times 128$ grid points is in very good agreement with the $256 \times 256$ grid point calculation. The number of bosons is $N = 10$ and the interaction strength $\Lambda = 0.1$. The bent parameters are $B = 2.5$, $D = 5.0$, and $a = 7.0$. The color codes are explained in each panel. The quantities shown are dimensionless.

As an additional measure to assess convergence and side by side, to explore complementary aspects of the dynamics of the system, we analyze the evolution of several key observables. Specifically, we track the variances in both position and momentum space, along with the expectation value and variance of the angular momentum operator. We focus on the variances as they are very sensitive to the many-body effects [8, 9]. All analyses are presented for calculations using $M = 4$ and $M = 8$ orbitals and also on $128 \times 128$ and $256 \times 256$ grids to demonstrate convergence of the calculated quantities.

Figure S5(a) and (b) present the position variances along the x- and y-directions, respectively. Panel (a) compares results obtained using $M = 4$ and $M = 8$ orbitals, while panel (b) shows simulations performed utilizing $128 \times 128$ and $256 \times 256$ grid points. In all cases, the data from the higher-resolution configurations lie directly on top of those from the lower-resolution setups, demonstrating that $M = 4$ orbitals and a $128 \times 128$ grid are sufficient to accurately capture the dynamics. A similar convergence behavior is observed for the momentum variances in both directions as well as for the angular momentum variances, as shown in Fig. S5(c), (d), and (f).

During the transport process, the momentum variance in both directions remains nearly constant, indicating that the dynamics are governed by position-space evolution with minimal momen-

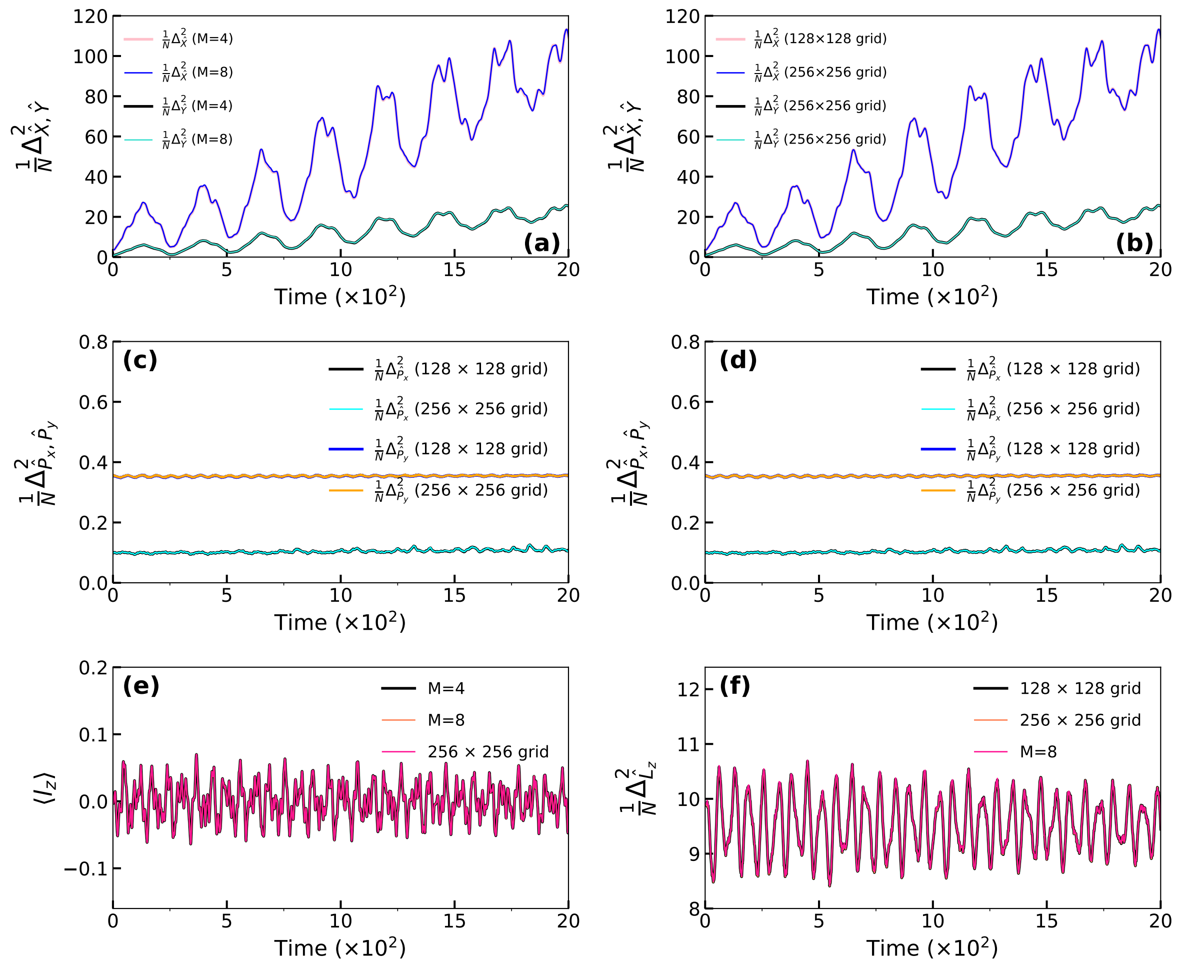


FIG. S5. $(a, b)$ Position variances in the x-direction ($\frac{1}{N}\Delta^2_{\hat{X}}$) and y-directions ($\frac{1}{N}\Delta^2_{\hat{Y}}$); $(c, d)$ momentum variances in x-direction ($\frac{1}{N}\Delta^2_{\hat{P}_x}$) and y-directions ($\frac{1}{N}\Delta^2_{\hat{P}_y}$); $(e)$ average angular momentum ($\langle l_z \rangle$); $(f)$ variance of the angular momentum ($\frac{1}{N}\Delta^2_{\hat{L}_z}$). Comparisons are made separately between $M = 4$ and $M = 8$ time-adaptive orbitals, and between grid resolutions of $128 \times 128$ and $256 \times 256$. The very close agreement confirms that combination of $M = 4$ orbitals and $128 \times 128$ grid are sufficient for converged results. Calculations are done for $N = 10$ bosons, interaction strength $\Lambda = 0.1$, and the bent parameters are $B = 2.5$, $D = 5.0$, and $a = 7.0$. Color codes are mentioned in each panel. All quantities are dimensionless.

tum redistributions. Furthermore, the angular momentum exhibits small oscillations around zero, signifying the absence of any net angular momentum transfer throughout the transport. However, this quantity represents the average angular momentum per particle. As mentioned earlier, in the mean-field calculation the particle number $N$ can be taken arbitrarily large while keeping $\Lambda$ fixed. Consequently, it is possible to generate a large total angular momentum by considering a

sufficiently large number of bosons.

---

[1] O. Penrose and L. Onsager, *Bose-Einstein condensation and liquid helium*, Phys. Rev. **104**, 576 (1956).

[2] K. Sakmann, A. I. Streltsov, O. E. Alon, and L. S. Cederbaum, *Universality of fragmentation in the Schrödinger dynamics of bosonic Josephson junctions*, Phys. Rev. A **89**, 023602 (2014).

[3] A. I. Streltsov, L. S. Cederbaum, and N. Moiseyev, *Ground-state fragmentation of repulsive Bose-Einstein condensates in double-trap potentials*, Phys. Rev. A **70**, 053607 (2004).

[4] R. Roy, A. Gammal, M. C. Tsatsos, B. Chatterjee, B. Chakrabarti, and A. U. J. Lode, *Phases, many-body entropy measrlres, and coherence of interacting bosons in optical lattices*, Phys. Rev. A **97**, 043625 (2018).

[5] O. E. Alon, A. I. Streltsov, and L. S. Cederbaum, *Multiconfigurational time-dependent Hartree method for bosons: Many-body dynamics of bosonic systems*, Phys. Rev. A **77**, 033613 (2008).

[6] R. Roy, S. Dutta, and O. E. Alon, *Rotation quenches in trapped bosonic systems*, Sci. Rep. **15**, 27193 (2025).

[7] A. U. J. Lode, C. Lévêque, L. B. Madsen, A. I. Streltsov, and O. E. Alon, *Colloquium: Multiconfigurational time-dependent Hartree approaches for indistinguishable particles*, Rev. Mod. Phys. **92**, 011001 (2020).

[8] S. Klaiman and O. E. Alon, *Variance as a sensitive probe of correlations*, Phys. Rev. A **91**, 063613 (2015).

[9] O. E. Alon, *Condensates in annuli: dimensionality of the variance*, Mol. Phys. **117**, 2108 (2019).
